# Supplementary material for: Reducing Disorder: An Information-Theory Formulation of MEV
Source: arXiv:2311.05367 source file (2023-11-09)
Supplement: Supplementary file 1 [file appendices.tex]

%% ---------------------------
%% If there is anything you would like to insert *after* the bibliography
%% (and *before* the \end{document} instruction), place it here
%% ---------------------------

% Nothing
